# Supplementary material for: Spiking Dynamics in Dual Free Layer Perpendicular Magnetic Tunnel Junctions
Source: arXiv:2309.07535 source file (2023-09-14)
Supplement: Supplementary file 1 [file Supplementary.pdf]

# SUPPLEMENTARY MATERIAL

# Spiking dynamics in dual free layer perpendicular magnetic tunnel junctions


L. Farcis,[*,†] B.M.S. Teixeira,[†] P. Talatchian,[†] D. Salomoni,[†] U. Ebels,[†] S. Auffret,[†] B. Dieny,[†] A. Mizrahi,[‡] J. Grollier,[‡] R.C. Sousa,[†] and L.D. Buda-Prejbeanu[†]

†*Univ. Grenoble Alpes, CEA, CNRS, Grenoble-INP, SPINTEC, 38000 Grenoble, France*

‡*Unité Mixte de Physique CNRS/Thales, Université Paris-Saclay, 91767 Palaiseau, France*

E-mail: louis.farcis@cea.fr


## Supplementary 1 : Macrospins model & parameters

Our model describing the magnetization dynamics of the two coupled macrospins, the soft (SL) and the hard (HL) layer, solves the Landau–Lifshitz–Gilbert-Slonczewski equation[1,2] (Eq. 1). The contribution from the demagnetizing field $\mathbf{H_{demag}}$, the anisotropy field $\mathbf{H_{anis}}$, the external magnetic field $\mathbf{H_{ext}}$, the spin-torque $\mathbf{H_{ST}}$, the dipolar field $\mathbf{H_{dip}}$ and the thermal field $\mathbf{H_{th}}$ are combined in the effective field $\mathbf{H_{eff}}$ (Eq. 2). The spin transfer torque is accounted through a damping-like term.

$$\frac{\partial \mathbf{m_i}}{\partial t} = -\frac{\gamma_0}{(1+\alpha^2)}\Big(\mathbf{m_i} \times \mathbf{H_{eff_i}} + \alpha \mathbf{m_i} \times (\mathbf{m_i} \times \mathbf{H_{eff_i}})\Big), \ for\ i \in \text{[SL,HL]} \tag{1}$$

$$\mathbf{H_{eff_i}} = \mathbf{H_{demag,i}} + \mathbf{H_{anis,i}} + \mathbf{H_{ext,i}} + \mathbf{H_{ST,i}} + \mathbf{H_{dip,i}} + \mathbf{H_{th,i}} \tag{2}$$

$$\mathbf{H_{ST,i}} = \frac{\hbar}{-2e}\frac{\eta}{\mu_0 M_{s,i} t_i}\frac{V}{R_p S}(\mathbf{m_i} \times \mathbf{m_j}); \text{ with } \eta = \frac{\sqrt{TMR(TMR+2)}}{2(TMR+1)} \tag{3}$$

The heat equation (Eq. 4) describes the temperature of the device to take into account the Joules heating[3] when the voltage bias is applied to the device where C and Q are the heat capacity and the thermal conductivity respectively. In addition, the anisotropies and the saturation magnetizations depend on the temperature through the Callen-Callen law (Eq. 5, 6).

$$C\frac{dT}{dt} + Q(T - T_0) = \frac{V^2}{R} \tag{4}$$

$$M_s(T) = M_{s0}\Big(1 - \Big(\frac{T}{T_c}\Big)^{1.73}\Big) \tag{5}$$

$$K_u(T) = K_{u0}\Big(\frac{M_s(T)}{M_{s0}}\Big)^2 \tag{6}$$

The following table summarizes the parameters used in the simulations :

| Parameters | Symbol | Values | Units |
|---|---|---|---|
| Saturation magnetization of SL at 300 K | $M_{s,SL}$ | 1250 | $A.m^{-1}$ |
| Saturation magnetization of HL at 300 K | $M_{s,HL}$ | 1250 | $A.m^{-1}$ |
| Uniaxial anisotropy of SL at 300 K | $K_{u,SL}$ | 703.5 | $kJ.m^{-3}$ |
| Uniaxial anisotropy of HL at 300 K | $K_{u,HL}$ | 1172.5 | $kJ.m^{-3}$ |
| damping of SL and HL | $\alpha$ | 0.113 | - |
| SL and HL geometry | $L_x \times L_y \times t$ | $80 \times 80 \times 1.1$ | $nm^3$ |
| Initial temperature | $T_0$ | 300 | $K$ |
| Tunnel magnetoresistance | $TMR$ | 32 | % |
| Resistance.Area product | $RA$ | 9.0 | $\Omega.\mu m^2$ |
| Simulation time step | $\delta t$ | $2 \times 10^{-13}$ | sec. |
| Heat capacity | $C$ | $1.510^{-6}$ | $V^2.s.K^{-1}.\Omega^{-1}$ |
| Thermal conductivity | $Q$ | $1.510^{-14}$ | $V^2.K{-}1.\Omega^{-1}$ |

# Supplementary 2 : Electrical characterization of Magnetic Tunnel Junctions

As mentioned in the main text, several MTJ devices shows stronger asymmetry between the effective anisotropy of the 2 layers. It results in 2 distinct coercive fields near zero bias and 2 different critical switching voltage as attested by the phase diagram Fig S2. When overpassing the critical voltage of the SL in the negative polarity (ie. $V_{c,SL} = -0.35V$), the reflected electron in the SL provide enough torque to stabilizes the AP state. It is only after crossing the critical voltage of the HL (ie. $V_{c,HL} = -0.48V$) that the windmill dynamic is generated.

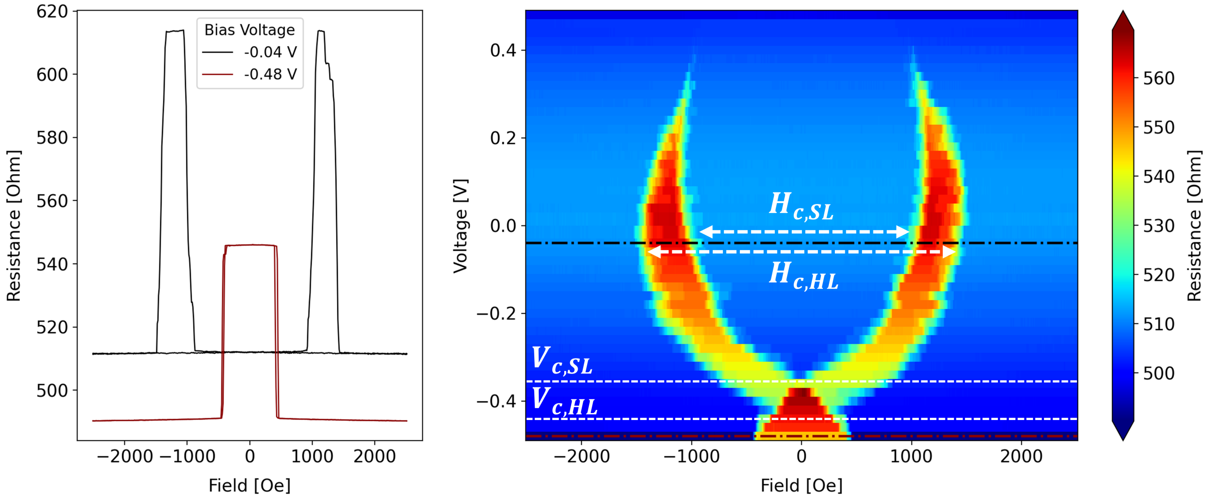


Figure 1: a) Resistance versus field loop of the MTJ nanopilar under -0.04 and -0.48 of voltage bias. b) Phase diagram extracted from R-H curves measurement for voltage bias from -0.48 to 0.48 V. The color code represent the average MTJ resistance during the sweeps up and down of the perpendicular magnetic field.

# References

(1) Landau, L.; Lifshitz, E. In *Perspectives in Theoretical Physics*; Pitaevski, L. P., Ed.; Pergamon: Amsterdam, 1992; pp 51–65.

(2) Slonczewski, J. Current-driven excitation of magnetic multilayers. *Journal of Magnetism and Magnetic Materials* **1996**, *159*, L1–L7.

(3) Strelkov, N.; Chavent, A.; Timopheev, A.; Sousa, R. C.; Prejbeanu, I. L.; Buda-Prejbeanu, L. D.; Dieny, B. Impact of Joule heating on the stability phase diagrams of perpendicular magnetic tunnel junctions. *Physical Review B* **2018**, *98*, 214410.
